# Supplementary material for: Approximate Dynamic Programming with Probabilistic Temporal Logic Constraints
Source: arXiv:1810.02199 source file (2018-10-05)
Supplement: Supplementary file 1 [file appendix.tex]

\subsection{Derivation of gradient}

\begin{align*}
\nabla_{\theta}\ell(s_{0}; \theta)
& \approx \nabla_{\theta}\left[ \sum_{z} p(z; \theta \mid s_{0}) \indicator \{D(s_{0}) \geq \beta \} - \alpha\right] \\
& = \sum_{z} \nabla_{\theta}p(z; \theta \mid s_{0}) \indicator \{D(s_{0}) \geq \beta \} \\
& = \sum_{z} p(z; \theta \mid s_{0}) \nabla_{\theta} \log{p(z; \theta \mid s_{0})} \indicator \{D(s_{0}) \geq \beta \} \\
& \approx \frac{1}{|Z|} \sum_{z} \nabla_{\theta} \log{p(z; \theta \mid s_{0})} \indicator \{D(s_{0}) \geq \beta \} \\
& = \frac{1}{|Z|} \sum_{z}[\sum_{t=0}^{T} \nabla_\theta \log \pi(a_t \mid s_t; \theta)]\indicator \{D(s_{0}) \geq \beta \} \\
% & = \frac{1}{|Z|} \sum_{z}\sum_{t=0}^{T} \frac{1}{\tau}[\phi(s_t,a_t) - \nabla_{\theta}V(s; \theta)]\indicator \{D(s_{0}) \geq \beta \}
\end{align*}

\begin{align*}
B(\ell(s_{0}; \theta))
& \approx B\left[ \sum_{z} p(z; \theta \mid s_{0}) \indicator \{D(s_{0}) \geq \beta \} - \alpha\right] \\
& = \max (\sum_{z} p(z; \theta \mid s_{0}) \indicator \{D(s_{0}) \geq \beta \} - \alpha, 0) \\
& \approx \max ( \frac{1}{|Z|} \sum_{z}\indicator \{D(s_{0}) \geq \beta \} - \alpha, 0)
\end{align*}

\subsection{Difference between \ac{adp} and \ac{pcl}}

In the \ac{pcl}, they first define a notion of soft consistency for a $d$-length sub-trajectory $s_{0:T} = (s_{0}, a_{0},\dots, s_{T-1}, a_{T-1}, s_{T})$ as a function of $\theta$:
\begin{equation*}
C(s_{0:T}; \theta) = -V(s_{0}; \theta) + \gamma^T V(s_{T}; \theta) + \sum_{t=0}^{T-1} \gamma^t [r(s_{t},a_{t}) - \tau \log \pi(a_{t} \mid s_{t}; \theta)]
\end{equation*}
The goal of a learning algorithm can then be to find to $V(\cdot; \theta)$ and $\pi(\cdot \mid \cdot; \theta)$ such that $C(s_{0:T}; \theta)$ is as close to 0 as possible as possible for all sub-trajectories $s_{0:T}$. Accordingly, we propose a new learning algorithm, called \ac{pcl}, that attempts to minimize the squared soft consistency error over a set of sub-trajectories $E$,
\begin{align*}
& \mbox{minimize} \qquad \underset{s_{0:T} \in E}{\sum} \frac{1}{2}\|V^{\ast} - \Phi \Theta\|^2
\end{align*}
In other words, the \ac{pcl} tries to minimize the squared softmax consistency error between the approximation and the true value $V^{\ast}$.
In terms of the Unified \ac{pcl}, the update rule for $\theta$ takes the form,
\begin{align*}
\triangle \theta = & \eta_{\pi} C(s_{0:T}; \theta)\sum_{t=0}^{T-1} \gamma^{t} \nabla_{\theta} \log \pi(a_{t} \mid s_{t}; \theta) + \\
& \eta_{v} C(s_{0:T}; \theta) (\nabla_{\theta} V(s_{t}; \theta) - \gamma^{t}\nabla_{\theta}V(s_{t}; \theta))
\end{align*}

In the \ac{adp} formulation, by the lemma~\ref{lm:1}, we can show that \ac{adp} tries to solve the similar problem but with one more extra constraint.
\begin{align*}
& \mbox{minimize} \qquad \underset{s_{0:T} \in E}{\sum}\|V^{\ast} - \Phi \Theta\| \\
& \mbox{subject to:} \ \ \ \ \calB \Phi \Theta \leq \Phi \Theta
\end{align*}
Moreover, since we use on-line sampling to get the sub-trajectories $s_{0: T} \in E$ to simulate the system by using the transitional probability matrix, the steady-state distribution $c$ can be captured~\cite{tsitsiklis1997analysis}, which is experimentally demonstrated to be convergent in section~\ref{sec:exp}. In other words, on-line sampling plays a very important role in this algorithm, in \cite{tsitsiklis1997analysis} they show that if the algorithm samples according to an arbitrary distribution which is independent of the state, the approximation of the value and the parameters both diverge to the infinity.

There are some advantages to \ac{lp}. First, the if both algorithms are trying to solve the same problem, the second one can achieve a better quality solution. Because of the inexact minimization, \ac{lp} formulation can ensure that constraint is not violated given the proper choice of the penalty. First, by adding extra constraints, the algorithm can be guided towards the global minimum and find a feasible solution just during the first one or two iterations of the algorithm. Second, we can cooperate with some system-level specifications by directly adding more constraints.

\begin{theorem}
	The solution of Randomized ADP is the optimal parameter for policy and value functions.
\end{theorem}

In the \ac{elp}, for any vector with positive components, minimizing $c^{\intercal}V$ yields $V^{\ast}$. In other words, the choice of state-relevance weights does not influence the solution. The same statement does not hold for the \ac{adp}.
\begin{lemma}
	A vector $\Tilde{r}$ solves
	\begin{align*}
	& \mbox{minimize} \qquad c^{\intercal}\Phi \Theta \\
	& \mbox{subject to:} \ \ \ \ \calB \Phi \Theta \leq \Phi \Theta
	\end{align*}
	if and only if it solves
	\begin{align*}
	& \mbox{minimize} \qquad \|V^* - \Phi \Theta\|_{1,c} \\
	& \mbox{subject to:} \ \ \ \ \calB \Phi \Theta \leq \Phi \Theta
	\end{align*}
	\label{lm:1}
\end{lemma}
\begin{proof}
	It is well known that the dynamic programming operator $\calB$ has the contraction property.  So $\calB$ is monotonic with the fixed point $V^\ast$, it follows that for any $V$ with $V \geq \calB V$, we have
	\begin{equation*}
	V \geq \calB V \geq \calB^2V \dots \geq \calB^n V \geq \dots \geq V^\ast
	\end{equation*}
	Hence, any $\theta$ that is a feasible solution to the optimization problems of interest satisfies $\Phi \Theta \geq V^{\ast}$. It follows that
	\begin{align*}
	\|V^\ast - \Phi \Theta\|_{1,c} = \underset{s \in S}{\sum}c(s)|V^\ast(s)-(\Phi\theta)(s)| \\
	= c^{\intercal} V^\ast - c^{\intercal}\Phi \Theta
	\end{align*}
	and minimizing $c^{\intercal}\Phi \Theta$ is therefore equivalent to minimizing $\|V^\ast - \Phi \Theta\|_{1,c}$.
\end{proof}

\section{Approximation}

\begin{theorem}
	(Weierstrass Approximation theorem) If $f$ is a continuous real-valued function defined over a real interval $[a,b]$. For every $\epsilon > 0$, there exists a polynomial $g$ such that:
	\begin{equation*}
	|f(x)-g(x)| < \epsilon, \text{ for all }x \in [a,b]
	\end{equation*}
	or equivalently, the supremum norm:
	\begin{equation*}
	\|f-g\| < \epsilon
	\end{equation*}
	\label{theorem:weierstrass}
\end{theorem}

\section{Error bound}

\begin{theorem}
	Let $e$ be in the span of the columns of $\Phi$ and $c$ be a probability distribution. Then, if $\Tilde{\theta}$ is an optimal solution to the \ac{adp},
	\begin{equation*}
	\|V^\ast - \Phi \Tilde{\theta}\|_{1,c} \leq \frac{2}{1-\gamma}\underset{\theta}{\min}\|V^\ast-\Phi \Theta\|_{\infty}
	\end{equation*}
\end{theorem}
\begin{proof}
	Let $\theta^\ast$ be one of the vectors minimizing $\|V^\ast - \Phi \Theta\|_{\infty}$ and define $\epsilon = \|V^\ast - \Phi \Theta^\ast \|_{\infty}$. The first step is to find a feasible point $ar{\theta}$ such that $\Phi ar{\theta}$ is within distance $O(\epsilon)$ of $V^\ast$. Because
	\begin{equation*}
	\|\calB\Phi \Theta^\ast - V^\ast\|_{\infty} \leq \gamma \|\Phi \Theta^\ast - V^\ast\|_{\infty}
	\end{equation*}
	
	\begin{align*}
	\|\calB \Phi \Theta^\ast - \calB V^\ast \|_{\infty} = & \underset{s \in S}{\max}| \underset{\pi}{\max}\{r(s, a) + \gamma \Expect_{s'} \Phi \Theta^\ast(s')\} - \calB V^\ast| \\
	& \leq | \underset{\pi}{\max}\{r(s^\ast,a) + \gamma \Expect_{s'} \Phi \Theta^\ast(s')\} - \calB V^\ast| \\
	& \leq |\{r(s^\ast,a^\ast) + \gamma \Expect_{s'} \Phi \Theta^\ast(s')\} - (r(s^\ast,a^\ast) + \gamma \Expect_{s'} V^\ast(s'))| \\
 	& = | \gamma \Expect_{s'} \Phi \Theta^\ast(s') - \gamma \Expect_{s'} V^\ast(s')|\\
 	& = \gamma | \Expect_{s'} \Phi \Theta^\ast(s') - \Expect_{s'} V^\ast(s')| \\
 	& = \Expect_{s'} \gamma|\Phi \Theta^\ast(s') -  V^\ast(s')| \\
 	& \leq \Expect_{s'} \gamma|\Phi \Theta^\ast(s^\ast) -  V^\ast(s^\ast)| \\
	& = \gamma|\Phi \Theta^\ast(s^\ast) -  V^\ast(s^\ast)| \underset{s'}{\sum} p(s' \mid s^\ast,a^\ast) \\
	& = \gamma|\Phi \Theta^\ast(s^\ast) -  V^\ast(s^\ast)|\\
	& \leq \gamma \|\Phi \Theta^\ast - V^\ast\|_{\infty}
 	\end{align*}
	where $a = \pi(\cdot \mid s)$
	
	Then we have
	\begin{equation}
	\calB \Phi \Theta^\ast \geq V^\ast - \gamma \epsilon e
	\label{eqn:error_1}
	\end{equation}
	We also recall that for any vector V and any scalar k,
	\begin{equation}
	\begin{split}
	\calB(V- k e) & = \underset{a}{\max}\{r_{u} + \gamma                   p_{a}(V- k e)\} \\
	& = \underset{a}{\max}\{r_u + \gamma p_{a}V-\gamma k e\} \\
	& = \underset{a}{\max}\{r_u + \gamma p_{a}V\} - \gamma k e \\
	& = \calB V - \gamma k e
	\label{eqn:error_2}
	\end{split}
	\end{equation}
	Combing \ref{eqn:error_1} and \ref{eqn:error_2}, we have
	\begin{align*}
	\calB(\Phi \Theta^\ast - k e) & = \calB\Phi \Theta^\ast - \gamma k e \\
	& \geq V^\ast - \gamma \epsilon e - \gamma k e \\
	& \geq \Phi \Theta^\ast - (1+\gamma) \epsilon e - \gamma k e   \\
	& = \Phi \Theta^\ast - k e + [(1-\gamma)k-(1+\gamma)\epsilon]e
	\end{align*}
	Because $e$ is within the span of the columns of $\Phi$, there exists a vector $ar{\theta}$ such that
	\begin{equation*}
	\Phi ar{\theta} = \Phi \Theta^\ast - \frac{(1+\gamma)\epsilon}{1-\gamma}e
	\end{equation*}
	and $ar{\theta}$ is a feasible solution to the \ac{adp}. By the triangle inequality,
	\begin{figure}
		\centering
		\includegraphics[width = \textwidth / 2]{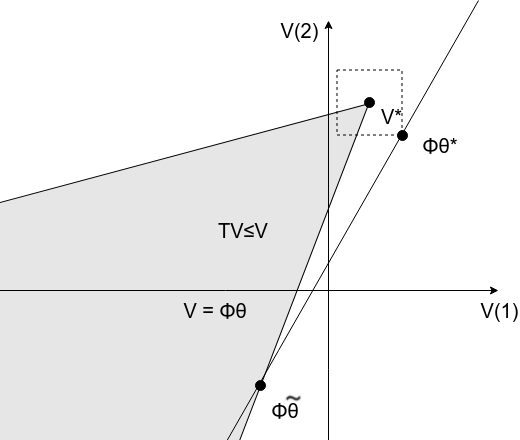}
		\caption{Graphical interpretation of approximation linear programming.}
		\label{fig:approximation}
	\end{figure}
	
	\begin{align*}
	\|\Phi ar{\theta} - V^\ast\|_{\infty} & \leq \|V^\ast - \Phi \Theta^\ast \|_{\infty} + \|\Phi \Theta^\ast - \Phi ar{\theta}\|_{\infty} \\
	& = \|V^\ast - \Phi \Theta^\ast\|_{\infty} + \frac{(1+\gamma)\epsilon}{1-\gamma}e \\
	& = \epsilon + \frac{(1+\gamma)\epsilon}{1-\gamma} \\
	& = \epsilon(1+\frac{1+\gamma}{1-\gamma}) = \frac{2\epsilon}{1-\gamma}
	\end{align*}
	If $\Tilde{\theta}$ is an optimal solution to the \ac{lp}, by \ref{lm:1} we have
	\begin{align*}
	\|V^\ast - \Phi \Tilde{V}\|_{1,c} & \leq\|V^\ast - \Phi ar{\theta}\|_{1,c} \\
	& \leq \|V^\ast - \Phi ar{\theta}\|_{\infty} \\
	& = \frac{2\epsilon}{1-\gamma}
	\end{align*}
	where the second inequality holds because $v$ is a probability distribution. The result follows.
\end{proof}
There are some significant weaknesses:
\begin{itemize}
	\item The bound calls for an element of the span of the basis functions to exhibit uniformly low error over all
	states. In practice, however, $\underset{\theta}{\min} \|V^\ast - \Phi \Theta\|$ is typically huge, especially for large-scale problems.
	\item The bound does not take into account the choice of state-relevance weights. As demonstrated in the previous section, these weights can significantly impact the approximation error. A sharp bound should take them into account.
\end{itemize} \cite{de2003linear}
